# Supplementary material for: Anisotropic optics and gravitational lensing of tilted Weyl fermions
Source: arXiv:2210.16145 ancillary file (2022-10-28)
Supplement: Supplementary file 1 [file Supplemental_Material.pdf]

# Supplemental Material - Anisotropic optics and gravitational lensing of tilted Weyl fermions

Viktor Könye,<sup>1</sup> Lotte Mertens,<sup>1,2</sup> Corentin Morice,<sup>3</sup> Dmitry Chernyavsky,<sup>1</sup>  
Ali G. Moghaddam,<sup>4,5</sup> Jasper van Wezel,<sup>2</sup> and Jeroen van den Brink<sup>1,6</sup>

<sup>1</sup>*Institute for Theoretical Solid State Physics, IFW Dresden and Würzburg-Dresden  
Cluster of Excellence ct.qmat, Helmholtzstr. 20, 01069 Dresden, Germany*

<sup>2</sup>*Institute for Theoretical Physics, University of Amsterdam,  
Science Park 904, 1098 XH Amsterdam, The Netherlands*

<sup>3</sup>*Laboratoire de Physique des Solides, CNRS UMR 8502,  
Université Paris-Saclay, F-91405 Orsay Cedex, France*

<sup>4</sup>*Department of Physics, Institute for Advanced Studies in Basic Sciences (IASBS), Zanjan 45137-66731, Iran*

<sup>5</sup>*Computational Physics Laboratory, Physics Unit,  
Faculty of Engineering and Natural Sciences, Tampere University, FI-33014 Tampere, Finland*

<sup>6</sup>*Institute for Theoretical Physics, TU Dresden, 01069 Dresden, Germany*

(Dated: October 28, 2022)

In this supplemental material we detail calculations of classical optical paths with Fermat's principle, compare geodesics obtained in Schwarzschild and Painlevé-Gullstrand coordinates, and present the details of the setup used for the current density calculation.

## I. EIKONAL APPROXIMATION

For the completeness of the paper, we will include a discussion on Fermat's principle of light in an inhomogeneous medium [1] and electrons in an inhomogeneous potential [2]. With this formalism, we extend the discussion to the details of the calculation of Weyl semimetals with inhomogeneous tilt.

### A. Light in medium with inhomogeneous refractive index

When considering rays of light in a medium, we can consider different properties of the waves such as the frequency, momentum, group velocity, and the refractive index. Starting from the Eikonal equation, we will consider these quantities.

#### 1. Eikonal approximation

For the known homogeneous case of light in a medium, we start with the wave equation

$$\partial_t^2 \Phi = c^2 \nabla^2 \Phi, \quad (1)$$

with the usual plane wave solutions

$$\Phi = A e^{i(\mathbf{k} \cdot \mathbf{r} - \omega t)}. \quad (2)$$

The relation between the frequency  $\omega$  and wave vector  $k$  is

$$\omega = ck, \quad (3)$$

with  $c$  the speed of light. In an inhomogeneous medium, the speed of light is not constant such that we get the

inhomogeneous wave equation

$$\partial_t^2 \Phi = c^2(\mathbf{r}) \nabla^2 \Phi. \quad (4)$$

We use the following ansatz for the form of the solutions

$$\Phi = A(\mathbf{r}, t) e^{i\varphi(\mathbf{r}, t)}, \quad (5)$$

and assume that the amplitude  $A$  is only slowly varying. The information is mainly carried in the quickly changing phase  $\varphi$ . We also neglect all second-order derivatives. With these assumptions, the wave equation becomes

$$(\partial_t \varphi)^2 = c^2(\mathbf{r}) |\nabla \varphi|^2. \quad (6)$$

We can further simplify this equation assuming the frequency of the light  $\omega$  is constant at all times:  $\varphi = -\omega t + \psi(\mathbf{r})$ . This gives

$$\omega^2 = c^2(\mathbf{r}) |\nabla \psi|^2. \quad (7)$$

This result can be compared with the plane wave ansatz of Eq. (2) such that we identify

$$\omega = -\partial_t \varphi, \quad \mathbf{k} = \nabla \varphi. \quad (8)$$

Inserting these definitions in Eq. (7) the *Eikonal equation* takes the form

$$\omega = c(\mathbf{r}) k. \quad (9)$$

#### 2. Momentum

We can rewrite Eq. (9) to obtain the wave vector as

$$k = \frac{\omega}{c(\mathbf{r})} = \frac{\omega n(\mathbf{r})}{c_0}, \quad (10)$$

where  $n(r)$  is the refractive index, and  $c_0$  is the speed of light in the vacuum. From Eq. (9) we can also calculate the local group velocity with

$$\mathbf{v} = \nabla_k \omega = c(\mathbf{r}) \frac{\mathbf{k}}{k}. \quad (11)$$

In this simple case, the group velocity is parallel to the wave vector which will simplify the later calculations.

### 3. Fermat's principle

Fermat's principle states that the trajectory of an optical path is stationary. This can represent a global or local minimum or maximum of the action. The optical path length is the line integral along the light rays between two points

$$\int \mathbf{k} d\mathbf{r}, \quad (12)$$

Optical paths that are close to each other will constructively interfere with each other. Thus, the actual optical path realized will be where the variation of the optical path length is zero. Using the results from the previous section

$$\begin{aligned} \delta \int \mathbf{k} d\mathbf{r} &= \delta \int k dl = 0, \\ \delta \int n dl &= 0, \end{aligned} \quad (13)$$

where we used the fact that the group velocity and the wave vector are parallel.

### 4. Path

In order to solve the variational problem of Eq. (13), we take a parametrization of the path,  $\mathbf{r}(w)$  with  $w$  an arbitrary parameter. Using this, the variational problem can be expressed as

$$\delta \int n(\mathbf{r}(w)) \sqrt{|\dot{\mathbf{r}}(w)|^2} dw = \delta \int L(\mathbf{r}(w), \dot{\mathbf{r}}(w)) dw = 0. \quad (14)$$

Where  $L$  is the *optical Lagrangian*. The Euler-Lagrange equation then is

$$\nabla L = \frac{d}{dw} \dot{\nabla} L, \quad (15a)$$

$$|\dot{\mathbf{r}}| \nabla n = \frac{d}{dw} \left( n \frac{\dot{\mathbf{r}}}{|\dot{\mathbf{r}}|} \right), \quad (15b)$$

where  $\dot{\nabla}$  is the derivative with respect to  $\dot{\mathbf{r}}$ . We use the commonly used arc-length parametrization [3, 4]  $w \rightarrow s = \int dl$ . With this  $|\dot{\mathbf{r}}| = 1$ . We define the following unit

vector  $\mathbf{e} = \dot{\mathbf{r}}$ . Using this the Euler-Lagrange equation simplifies to

$$\dot{\mathbf{e}} = \frac{(1 - \mathbf{e} \otimes \mathbf{e}) \nabla n}{n}. \quad (16)$$

Together with the equation  $\dot{\mathbf{r}} = \mathbf{e}$  this is a differential equation system that given the initial position and the initial direction uniquely defines the trajectory of the light ray.

## B. Electrons in inhomogeneous potential

After the introduction of all necessary tools to consider different optical systems, we expand the solution to electrons in an inhomogeneous potential.

### 1. Eikonal approximation

Similarly to the eikonal approximation for light we first look at the homogeneous system. The differential equation, in this case, is the Schrödinger equation

$$i\partial_t \Phi = H\Phi, \quad (17)$$

where

$$H = -\frac{\nabla^2}{2m}. \quad (18)$$

This has plane wave solutions as

$$\Phi = A(\mathbf{k}) e^{i(\mathbf{k} \cdot \mathbf{r} - Et)}, \quad (19)$$

with energy

$$E = \frac{k^2}{2m}. \quad (20)$$

We now introduce inhomogeneity using a potential as

$$H = -\frac{\nabla^2}{2m} + V(\mathbf{r}). \quad (21)$$

Which gives the wave equation

$$i\partial_t \Phi = -\frac{\nabla^2 \Phi}{2m} + V(\mathbf{r}) \Phi.$$

We can again use the following ansatz

$$\Phi = A(\mathbf{r}, t) e^{i\varphi(\mathbf{r}, t)}. \quad (22)$$

Using the same assumptions as we did for light ( $E \equiv \omega$ ) we get

$$E = \frac{k^2}{2m} + V(\mathbf{r}). \quad (23)$$

### C. Momentum

We can again rewrite Eq. (23) to get the wave vector

$$k = \sqrt{2m(E - V(\mathbf{r}))} = \sqrt{2m} n_{\text{eff}}(\mathbf{r}), \quad (24)$$

where  $n_{\text{eff}}$  can be thought of as an effective refractive index. From Eq. (23) we can also calculate the local group velocity which is

$$\mathbf{v} = \nabla_{\mathbf{k}} E = \frac{\mathbf{k}}{m}. \quad (25)$$

In this case, the group velocity is again parallel to the wave vector. Since the expression for the momentum is completely analogous to the case of light, the calculation of the trajectory is exactly the same and can be performed by using the effective refractive index.

### D. Weyl cones with inhomogeneous tilt

After constructing the basic results of eikonal approximation for optics and electrons subjected to an inhomogeneous potential, we can now introduce the same principles to a new system, i.e. Weyl semimetals with an inhomogeneous tilt.

#### 1. Eikonal approximation

Again we start from the Schrödinger equation

$$i\partial_t \Phi_\alpha = H_{\alpha\beta} \Phi_\beta, \quad (26)$$

with the Hamiltonian

$$H_{\alpha\beta} = -i(\sigma_{\alpha\beta}^j - t^j \delta_{\alpha\beta}) \partial_j. \quad (27)$$

with  $j \in (1, 2)$  the dimensional indices and  $\alpha, \beta \in (0, 1)$  the indices matrices. Again taking the plane wave ansatz

$$\Phi_\alpha = A_\alpha(\mathbf{k}) e^{i(\mathbf{k} \cdot \mathbf{r} - Et)}, \quad (28)$$

the equation becomes

$$EA_\alpha(\mathbf{k}) = H_{\alpha\beta}(\mathbf{k}) A_\beta(\mathbf{k}), \quad (29)$$

with the Hamiltonian

$$H_{\alpha\beta}(\mathbf{k}) = (\sigma_{\alpha\beta}^j - t^j \delta_{\alpha\beta}) k_j. \quad (30)$$

In this case, we introduce the inhomogeneity using a tilting parameter that is position dependent. The Hamiltonian becomes

$$H_{\alpha\beta}(\mathbf{r}) = -i \left[ \sigma_{\alpha\beta}^j - t^j(\mathbf{r}) \delta_{\alpha\beta} \right] \partial_j + i \frac{1}{2} \partial_j t^j(\mathbf{r}) \delta_{\alpha\beta}, \quad (31)$$

where the last term is needed for Hermiticity. Again the previous ansatz

$$\Phi_\alpha(\mathbf{r}, t) = A_\alpha(\mathbf{r}, t) e^{i\varphi(\mathbf{r}, t)}, \quad (32)$$

and the previous approximations give the eikonal equation

$$E = \pm k - t^j k_j. \quad (33)$$

Here we also assume that  $A_\alpha(\mathbf{r}, t)$  follows the local eigenvector in the upper or lower bands without any mixing between the two bands, or more specifically,  $\sigma_{\alpha\beta}^j k_j A_\beta = A_\alpha k$ . This means that the approximation strictly-speaking only works far away from the Weyl point. We also assumed small variations in the tilting parameter and thus neglected the derivative of the tilting parameter.

#### 2. Momentum

From now on we will only consider the upper band (calculations for the lower band can be done analogously)

$$E = E_+(\mathbf{k}, \mathbf{r}) = k - t^j k_j. \quad (34)$$

We assume the following radial position dependence for the tilting

$$t_j = \frac{r_j}{r} t(r). \quad (35)$$

The eikonal equation takes the following form

$$E = k - \frac{r^j k_j}{r} t(r). \quad (36)$$

The group velocity is

$$\mathbf{v} = \partial_{\mathbf{k}} E = \frac{\mathbf{k}}{k} - \frac{\mathbf{r}}{r} t(r). \quad (37)$$

We define the versors of  $\mathbf{r}$ ,  $\mathbf{k}$  and  $\mathbf{v}$  (see Fig. 1) as

$$\begin{aligned} \hat{\mathbf{r}} = \frac{\mathbf{r}}{r} &= \begin{pmatrix} \cos \varphi \\ \sin \varphi \end{pmatrix}, & \hat{\mathbf{k}} = \frac{\mathbf{k}}{k} &= \begin{pmatrix} \cos \alpha \\ \sin \alpha \end{pmatrix}, \\ \hat{\mathbf{v}} = \frac{\mathbf{v}}{v} &= \begin{pmatrix} \cos \vartheta \\ \sin \vartheta \end{pmatrix}. \end{aligned} \quad (38)$$

The norm of the velocity is

$$v^2 = 1 + t(r)^2 - 2t(r) \cos(\alpha - \varphi). \quad (39)$$

The velocity is

$$v\hat{\mathbf{v}} = \hat{\mathbf{k}} - \hat{\mathbf{r}}t(r), \quad (40)$$

using this equation the versor of the momentum is

$$\hat{\mathbf{k}} = v\hat{\mathbf{v}} + \hat{\mathbf{r}}t(r). \quad (41)$$

As we can see without tilt the momentum and the velocity are parallel but for arbitrary tiltings this is no longer the case. The angle  $\alpha$  can be calculated from Eq. (41) as an implicit equation

$$\cos \alpha = v \cos \vartheta + t \cos \varphi, \quad (42a)$$

$$\sin \alpha = v \sin \vartheta + t \sin \varphi. \quad (42b)$$

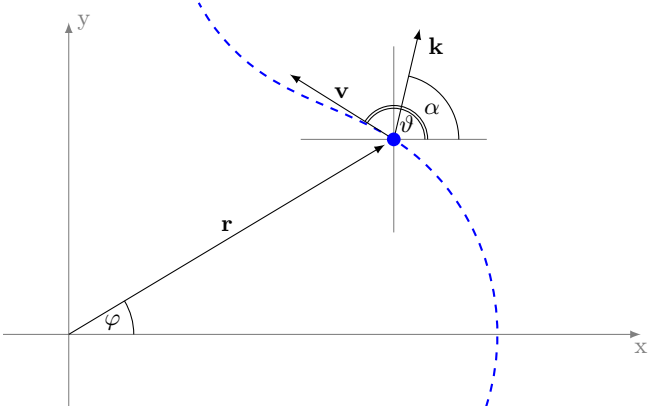

Figure 1. Definitions of vectors and angles.

Combining these two equations we can get

$$\cos(\alpha - \varphi) = v \cos(\vartheta - \varphi) + t. \quad (43)$$

Carefully considering the signs we can explicitly express  $\cos(\alpha - \varphi)$  as

$$\begin{aligned} \cos(\alpha - \varphi) &= t \sin^2(\vartheta - \varphi) + \\ &+ \cos(\vartheta - \varphi) \sqrt{1 - t^2 \sin^2(\vartheta - \varphi)}. \end{aligned} \quad (44)$$

Substituting this in the velocity

$$v = \sqrt{1 - t^2 \sin^2(\vartheta - \varphi)} - t \cos(\vartheta - \varphi). \quad (45)$$

Using the versors in Eq. (36) we get

$$E = k \left[ 1 - \hat{r}^j \hat{k}_j t(r) \right], \quad (46a)$$

$$E = k \left[ 1 - v \cos(\vartheta - \varphi) t(r) - t^2(r) \right]. \quad (46b)$$

This means that the magnitude of the momentum can be expressed as

$$k = \frac{E}{1 - v \cos(\vartheta - \varphi) t(r) - t^2(r)}. \quad (47)$$

Substituting  $v$  from Eq. (45) gives

$$k = \frac{E}{1 - t^2 \sin^2(\vartheta - \varphi) - t \cos(\vartheta - \varphi) \sqrt{1 - t^2 \sin^2(\vartheta - \varphi)}}. \quad (48)$$

### 3. Fermat's principle

Similarly to the case of light, we consider the following line integral along the trajectory

$$\int \mathbf{k} \, d\mathbf{r}. \quad (49)$$

Again, the criterion for constructive interference is

$$\delta \int \mathbf{k} \, d\mathbf{r} = \delta \int k \cos(\alpha - \vartheta) \, dl = 0, \quad (50a)$$

$$\delta \int n_{\text{eff}} \, dl = 0. \quad (50b)$$

The major difference compared to the previous cases is that now the effective refractive index depends on the direction of the group velocity ( $\vartheta$ ). Similarly to Eq. (43) we can write

$$\cos(\alpha - \vartheta) = v + t \cos(\varphi - \vartheta) = \sqrt{1 - t^2 \sin^2(\vartheta - \varphi)}. \quad (51)$$

Using this the effective refractive index becomes

$$n_{\text{eff}} = \frac{E}{v}. \quad (52)$$

### 4. Path

In order to solve the variational problem, we take an arbitrary parametrization of the path as  $\mathbf{r}(w)$ . Using this the variational problem can be expressed as

$$\begin{aligned} &\delta \int n(\mathbf{r}(w), \dot{\mathbf{r}}(w)) |\dot{\mathbf{r}}(w)| \sqrt{|\dot{\mathbf{r}}(w)|^2} \, dw \\ &= \delta \int L(\mathbf{r}(w), \dot{\mathbf{r}}(w)) \, dw = 0 \end{aligned} \quad (53)$$

where we renamed  $n_{\text{eff}}$  as  $n$ . The Euler-Lagrange equation of this is

$$\nabla L = \frac{d}{dw} \dot{\nabla} L, \quad (54a)$$

$$|\dot{\mathbf{r}}| \nabla n = \frac{d}{dw} \left( n \frac{\dot{\mathbf{r}}}{|\dot{\mathbf{r}}|} + |\dot{\mathbf{r}}| \dot{\nabla} n \right). \quad (54b)$$

Using the line element parametrization as before the Euler-Lagrange equation simplifies to

$$\nabla n = \frac{d}{ds} [\mathbf{e} n + (1 - \mathbf{e} \otimes \mathbf{e}) \nabla_e n], \quad (55)$$

Together with the equation  $\dot{\mathbf{r}} = \mathbf{e}$  this is a differential equation system that given the initial position and the initial direction uniquely defines the trajectory of the electron. It is important to note that these equations only give the spatial trajectory but have no information about the time it takes to go through these trajectories.

### 5. Trajectory with polar coordinates

Using the definitions in Eq. (38) we can express the trajectory equation Eq. (55) in polar coordinates. We start with the  $\dot{\mathbf{r}} = \mathbf{e}$  equation

$$\dot{x} = \cos \vartheta \quad \Rightarrow \quad \dot{r} \cos \varphi - r \sin \varphi \dot{\varphi} = \cos \vartheta, \quad (56a)$$

$$\dot{y} = \sin \vartheta \quad \Rightarrow \quad \dot{r} \sin \varphi + r \cos \varphi \dot{\varphi} = \sin \vartheta, \quad (56b)$$

combining the two equations we get

$$\dot{r} = \cos(\vartheta - \varphi), \quad (57a)$$

$$\dot{\varphi} = \frac{\sin(\vartheta - \varphi)}{r}. \quad (57b)$$

The derivatives in polar coordinates are

$$\nabla = \begin{pmatrix} \cos \varphi \partial_r - \frac{\sin \varphi \partial_\varphi}{r} \\ \sin \varphi \partial_r + \frac{\cos \varphi \partial_\varphi}{r} \end{pmatrix}, \quad \nabla_e = \begin{pmatrix} -\frac{\sin \vartheta \partial_\vartheta}{r} \\ \frac{\cos \vartheta \partial_\vartheta}{r} \end{pmatrix}. \quad (58a)$$

With this, Eq. (55) becomes

$$\cos \varphi \partial_r n - \frac{\sin \varphi \partial_\varphi n}{r} = \frac{d}{ds} [\cos(\vartheta) n - \sin(\vartheta) \partial_\vartheta n], \quad (59a)$$

$$\sin \varphi \partial_r n + \frac{\cos \varphi \partial_\varphi n}{r} = \frac{d}{ds} [\sin(\vartheta) n + \cos(\vartheta) \partial_\vartheta n]. \quad (59b)$$

The different derivatives are

$$\begin{aligned} \dot{n} &= \dot{r} \partial_r n + \dot{\varphi} \partial_\varphi n + \dot{\vartheta} \partial_\vartheta n \\ &= \cos(\vartheta - \varphi) \partial_r n + \frac{\sin(\vartheta - \varphi)}{r} \partial_\varphi n + \dot{\vartheta} \partial_\vartheta n, \end{aligned} \quad (60a)$$

$$\begin{aligned} (\partial_\vartheta \dot{n}) &= \dot{r} \partial_r \partial_\vartheta n + \dot{\varphi} \partial_\varphi \partial_\vartheta n + \dot{\vartheta} \partial_\vartheta^2 n \\ &= \cos(\vartheta - \varphi) \partial_r \partial_\vartheta n + \frac{\sin(\vartheta - \varphi)}{r} \partial_\varphi \partial_\vartheta n + \dot{\vartheta} \partial_\vartheta^2 n. \end{aligned} \quad (60b)$$

Using these and trigonometric transformations the equation for  $\vartheta$  becomes

$$\dot{\vartheta} = -\frac{\sin(\vartheta - \varphi) \left( \partial_r n + \frac{1}{r} \partial_\varphi \partial_\vartheta n \right) + \cos(\vartheta - \varphi) \left( \partial_r \partial_\vartheta n - \frac{1}{r} \partial_\varphi n \right)}{n + \partial_\vartheta^2 n}. \quad (61a)$$

With this equation and the form of  $t(r) = \sqrt{r_s/r}$  from the main paper we can find the effective refractive index for the Weyl cone system.

## II. BLACK HOLE ANALOGUE

As mentioned, the Hamiltonian model is analogous to a Schwarzschild black hole given in Painlevé-Gullstrand (PG) coordinates. The two models give the same Dirac equation for massless fermions. In this appendix, we will consider the exact geodesics and highlight the differences between the Schwarzschild metric and the PG metric for completeness.

The most general metric that the Hamiltonian maps to is

$$ds^2 = (t^2(r) - 1) dT^2 - 2t(r) dr dT + dr^2 + r^2 d\theta^2. \quad (62)$$

In the case of (1+2)D  $d\theta$  denotes polar angle differential, while for (1+3)-dimensional spacetime it corresponds to the line element on a two-dimensional sphere. Now, if we take

$$t^2(r) = \frac{2M}{r}, \quad (63)$$

the metric describes a Schwarzschild black hole with radius  $r_s = 2M$  written in the PG coordinates. This PG metric is closely related to the Schwarzschild metric. Only the time coordinate in the metric is changed to the proper time of a radially infalling observer with a transformation of the form  $T_r = T + a(r)$  [5]. The radial coordinate accordingly measures the proper distance between two radially infalling observers [5]. For both metrics we can consider the geodesics and causal structure and compare them to the Fermat results above.

### A. Geodesics

The Schwarzschild metric is given by

$$ds^2 = [t^2(r) - 1] dT_r^2 + \frac{dr^2}{t^2(r) - 1} + r^2 d\theta^2, \quad (64)$$

where

$$t^2(r) = \frac{2M}{r} = \frac{r_s}{r}. \quad (65)$$

As only the time coordinate changes from the Schwarzschild to the PG metric, the position coordinates (and thus the position of the black hole) stay the same. On both metrics, we can define two conserved quantities: energy ( $E$ ) and angular momentum ( $L$ ). With these we can find the geodesics. The result are given in Eq. (66) for Schwarzschild and Eq. (67) for the PG coordinate system.

$$\begin{aligned} E_r &= (r_s/r_0 - 1), \\ L &= r_0^2 \frac{d\theta}{d\tau} \Big|_0, \\ \frac{dt}{d\tau} &= \frac{E}{r_s/r - 1}, \\ \frac{dr}{dt} &= \pm \frac{d\tau}{dt} \sqrt{E^2 + L^2/r^2(r_s/r - 1)}, \\ \frac{d\theta}{dt} &= \frac{dt}{d\tau} \frac{L}{r^2}, \\ \frac{dr}{d\theta} &= \pm \frac{r^2}{L} \sqrt{E^2 + L^2/r^2(r_s/r - 1)}, \end{aligned} \quad (66)$$

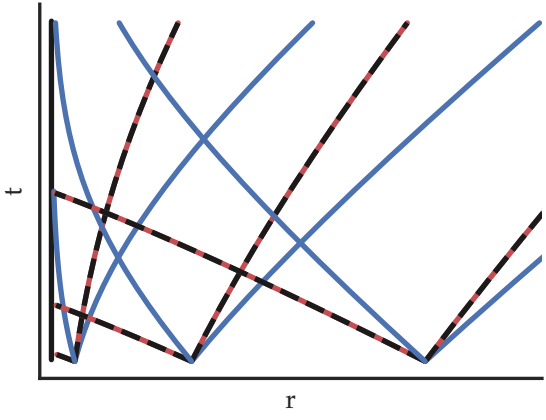

Figure 2. Comparison of spacetime diagrams of the Schwarzschild black hole for the two different metrics and zero angular momentum. The red lines are the Painlevé-Gullstrand coordinates and the blue lines the Schwarzschild coordinates. The dispersion relation of the Hamiltonian model (black) is derived from Eq. (37).

$$\begin{aligned}
E &= (r_s/r_0 - 1) \frac{dT}{d\tau} \Big|_0 - \sqrt{r_s/r} \frac{dr}{dT} \Big|_0, \\
L &= r_0^2 \frac{d\theta}{d\tau} \Big|_0, \\
\frac{dT}{d\tau} &= \frac{E + \sqrt{r_s/r} \frac{dr}{d\tau}}{r_s/r - 1}, \\
\frac{dr}{dT} &= \pm \frac{d\tau}{dT} \sqrt{E^2 + L^2/r^2(r_s/r - 1)}, \\
\frac{dr}{dT} &= \frac{(r_s/r - 1) \sqrt{E^2 + L^2/r^2(r_s/r - 1)}}{\pm E + \sqrt{r_s/r} \sqrt{E^2 + L^2/r^2(r_s/r - 1)}}, \\
\frac{d\theta}{dT} &= \frac{d\tau}{dT} \frac{L}{r^2}, \\
\frac{dr}{d\theta} &= \pm \frac{r^2}{L} \sqrt{E^2 + L^2/r^2(r_s/r - 1)}. \tag{67}
\end{aligned}$$

As one can see, the equations of the geodesics  $\frac{dr}{d\theta}$  are the same in the two metrics. The radial coordinate has not changed between the two frames. However, the geodesics' time dependence (and thus the velocity of light) has changed.

### B. Causal structure

This difference in velocity can be quantified by comparing the causal structure of the metrics as given in Fig. 2. Again the red line is from the PG metric, while the blue line is from the Schwarzschild metric. For Schwarzschild at  $r_s$ , both branches ( $\pm$ ) become zero at the horizon. For

the PG coordinates, however, only one band (the outgoing) will become zero and the other keeps a finite velocity infalling towards the black hole.

The black dashed lines are the dispersion relations for the low energy of the Hamiltonian model obtained from the low energy limit of the Weyl cones. However, the Weyl cones of a system can not be directly compared to light cones in the spacetime diagram. The Weyl cones are expressed with energy as a function of both momentum and position. At each position, a tilted Weyl cone is defined. To obtain a light cone, first, the derivative (slope) of the Weyl cone must be calculated. Next, instead of expressing  $k$  as a function of  $E$  we should take  $\partial_k E = v = \frac{dr}{dt}$  as the velocity in  $r, t$  space and integrate to obtain  $r$  as a function of  $t$ . Here we have taken the momentum solely in the radial direction, equivalent to  $L = 0$ .

For a dispersion relation that is linear in  $k$  (simplifying to 1D due to the radial velocity),  $E = f(r)k$  the cones are related and take the form

$$dr = f(r)dt \tag{68}$$

thus for the special case of a linear dispersion relation, the velocities are indeed proportional to the prefactor of the dispersion relation.

The resulting light cones from the Hamiltonian and the PG light cones are exactly the same. However, as the dispersion relation itself is an approximation, this is not the velocity for the wave packet in the full Hamiltonian. The velocities for the wave packet in the full Hamiltonian will therefore diverge from the lines in Fig. 2, as shown in the main text.

The former comparison shows that the qualitative behavior of light will be the same for both metrics. In both, we will see the lensing of light, equal to the predicted dispersion from Fermat's principle. Even though the velocity of particles along their spatial trajectories is different in the different metrics, the spatial trajectories themselves are exactly the same. The specific Hamiltonian with tilted Weyl cones that maps to the PG metric has been chosen because of its possible experimental implementation, while a Hamiltonian mapping onto the Schwarzschild metric itself would be harder to realize.

## III. CURRENT DENSITY SETUP

In this section, we show the setup for the current density calculations. The scattering setup is shown in Fig. 3 for a system of size  $20 \times 20$ . For the actual calculations we used a much larger system which is  $1000 \times 1000$ . The scattering region (blue) is connected to four leads from all sides. The lead on the left is split into two parts, with a smaller part on the top left corner (red). This lead is used to inject current for the current density calculation.

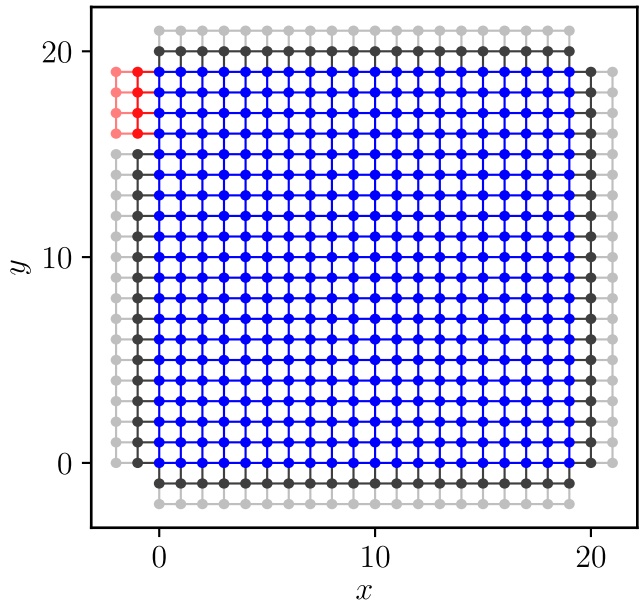

Figure 3. Scattering setup for current density calculations. Blue sites are the scattering region. Black sites are the leads connected to this. The red sites represent the lead that is used to inject current. The relative widths in this  $20 \times 20$  setup are the same as in the  $1000 \times 1000$  setup presented in the main paper.

- 
- [1] E. Born, Max and Wolf, *Principles of Optics*, 7th ed. (Cambridge University Press, 1999).
  - [2] H. van Houten and C. W. J. Beenakker, Principles of solid state electron optics, in *Confined Electrons and Photons: New Physics and Applications*, edited by E. Burstein and C. Weisbuch (Springer US, Boston, MA, 1995) pp. 269–303.
  - [3] A. L. Rivera, K. B. Wolf, and S. M. Chumakov, Hamiltonian foundation of geometrical anisotropic optics, *JOSA A*, Vol. 12, Issue 6, pp. 1380-1389 **12**, 1380 (1995).
  - [4] M. P. Rudzki, 2. on application of fermat's principle to anisotropic media, in *Anisotropy 2000* (Society of Exploration Geophysicists, 2001) pp. 13–20.
  - [5] R. Gautreau and B. Hoffmann, The schwarzschild radial coordinate as a measure of proper distance, *Physical Review D* **17**, 2552 (1978).
